# Supplementary material for: Nearly Tight Lower Bound for Range Minimum Query via Probe-by-Probe Information Accounting
Source: arXiv:2111.02318 source file (2026-10-17)
Supplement: Supplementary file 1 [file appendix.tex]

\ifx\mainfile\undefined
\documentclass[11pt]{article}
\input{macro}

\begin{document}
\fi

\section{Proof of \cref{claim: tail extent}}\label{sec: prove claim: tail extent}
	Note that $H(\foot_i(Q_{\pub})|\foot_{<i}(Q_{\pub}),\cK_i)\ge H(\foot_i(Q_{\pub})|\foot_{<i}(Q_{\pub}),\rest_i(Q_{\pub}))$ since $\cK_i$ is known from $\foot_{<i}(Q_{\pub})$ together with $\rest_i(Q_{\pub}),Q_{\pub}$.
	Thus it suffices to prove 
	\begin{align}
	H(\foot_i(Q_{\pub})|\foot_{<i}(Q_{\pub}),\rest_i(Q_{\pub}))= H(\foot_i(Q_{\pub})|\foot_{<i}(Q_{\pub}))-O(p\log B).\label{eq: encode arugment}
	\end{align}

	For any $i\in[t]$, the following encoding scheme always exists:
\begin{enumerate}[label=({\arabic*})]
	\item
		write down the $p$ published bits;
	\item
		write down $S_{\pt}$;
	\item
		sample $\Delta\in[L]$ uniformly at random, write down $\Delta$;
	\item
		write down the contents of cells in $\probe_{<i}(Q_{\pub})$ using $w\cdot|\probe_{<i}(Q_{\pub})|$ bits;
	\item
	  	write down the contents of cells in $\probe_{-i}(Q_{\pub})$, i.e. the contents of all the cells excluding the cells in $\probe_{\le i}(Q_{\pub})$, in the increasing order of their addresses, using $|\rest_i(Q_{\pub})|$ bits;
	\item
		write down the contents of the cells in $\probe_i(Q_{\pub})\setminus\probe_{<i}(Q_{\pub})$ in the increasing order of their addresses, using the optimal expected $H(\foot_{i}(Q_{\pub})\mid\rest_i(Q_{\pub}),\foot_{<i}(Q_{\pub}))$ bits.
  \end{enumerate}
  Recall that $Q_{\pub}$ is known from $S_{\pt}$ together with $\Delta$.
  It is easy to see that we can decode the whole data structure, together with all the published bits, from the codeword.
  Furthermore, we can decode the input database from the data structure, thus the codeword must be of length at least $H_{d,u,B,Z}$ bits in expectation.

  According to \cite[Proof of Lemma 4]{liu2020lower}, the first three steps consume $O(p\log B)$ bits.

  The encoding scheme partitions the set of all the cells of the data structure into three disjoint sets: $\probe_{<i}(Q_{\pub})$, $\probe_i(Q_{\pub})\setminus\probe_{<i}(Q_{\pub})$, and $\probe_{-i}(Q_{\pub})$.
  Note that the partition is known as long as the addresses together with the contents of the cells in $\probe_{<i}(Q_{\pub})$, i.e. $\foot_{<i}(Q_{\pub})$, are known.
   The data structure represents the contents of the cells in $\probe_i(Q_{\pub})\setminus\probe_{<i}(Q_{\pub})$ using $w\cdot\mathbb{E}[|\probe_i(Q_{\pub})\setminus\probe_{<i}(Q_{\pub})|]\ge H(\foot_{i}(Q_{\pub})\mid\foot_{<i}(Q_{\pub}))$ bits in expectation.
  On the other hand, the above encoding scheme represents the contents of the cells in $\probe_i(Q_{\pub})\setminus\probe_{<i}(Q_{\pub})$ using expected $H(\foot_{i}(Q_{\pub})\mid\rest_i(Q_{\pub}),\foot_{<i}(Q_{\pub}))$ bits at cost of writing down extra $O(p\log B)$ bits.
  If $H(\foot_{i}(Q_{\pub})\mid\foot_{<i}(Q_{\pub}))-H(\foot_{i}(Q_{\pub})\mid\rest_i(Q_{\pub}),\foot_{<i}(Q_{\pub}))=\omega(p\log B)$, the last step will save $\omega(p\log B)$ bits in writing down the contents of the cells in $\probe_i(Q_{\pub})\setminus\probe_{<i}(Q_{\pub})$.
  Which is impossible, since we do not waste any bit in writing down the contents of the cells in $\probe_{<i}(Q_{\pub})$ and $\probe_{-i}(Q_{\pub})$.
  In other words, the codeword is of length $H_{d,u,B,Z}-\omega(p\log B)$ bits in expectation, if Eq\eqref{eq: encode arugment} does not hold. %

  Therefore, $H(\foot_i(Q_{\pub})|\foot_{<i}(Q_{\pub}),\rest_i(Q_{\pub}))= H(\foot_i(Q_{\pub})|\foot_{<i}(Q_{\pub}))-O(p\log B)$.

\section{Proof of \cref{claim: condition manipulate}}\label{sec: prove claim: condition manipulate}
	Note that $H(\foot_{< i}(Q_{\pub})\mid \cK_i)\ge H(\foot_{< i}(Q_{\pub})\mid \cK_i,\cK_{i-1},\cK'_{i-1})$, and $H(\foot_{< i}(Q_{\pub})\mid \cK_{i-1})-H(\foot_{< i}(Q_{\pub})\mid \cK_i,\cK_{i-1},\cK'_{i-1})= I(\foot_{<i}(Q_{\pub}):\cK_{i},\cK'_{i-1}\mid \cK_{i-1})\le H(\cK_{i},\cK'_{i-1}\mid \cK_{i-1})$.

\section{Proof of \cref{fact: inequality}}\label{section: proof of fact}
\begin{align*}
	&\mathbb{E}[X\log(Y/X)]\\
	=&\mathbb{E}[Y(X/Y)\log(Y/X)]\\
	=&\sum_y\Pr[Y=y]\cdot y\cdot\mathbb{E}[(X/Y)\log(Y/X)\mid Y=y]\\
	\intertext{By the convexity of $x\log(1/x)$,}
	\le&\sum_y\Pr[Y=y]\cdot y\cdot\mathbb{E}[X/Y\mid Y=y]\log(1/\mathbb{E}[X/Y\mid Y=y])]\\ %
	=&\mathbb{E}[Y] \sum_y(\Pr[Y=y]\cdot y/\mathbb{E}[Y])\mathbb{E}[X/Y\mid Y=y]\log(1/\mathbb{E}[X/Y\mid Y=y])]
	\intertext{Observe that $(\Pr[Y=y]\cdot y/\mathbb{E}[Y])$ is a probability function with respect to $y$. Let $\mu$ denote the distribution,}
	=&\mathbb{E}[Y]\mathbb{E}_{y\sim\mu}[\mathbb{E}[X/Y\mid Y=y]\log(1/\mathbb{E}[X/Y\mid Y=y])]
	\intertext{Note that $\mathbb{E}_{y\sim\mu}[\mathbb{E}[X/Y\mid Y=y]]=\mathbb{E}[X]/\mathbb{E}[Y]$, by the convexity of function $x\log(1/x)$,}
	\le&\mathbb{E}[X]\log(\mathbb{E}[Y]/\mathbb{E}[X]).
\end{align*}

\section{Proof of \cref{lem_enc_len}}\label{section: lem_enc_lem}
First note that $\cK\subseteq\cE$.
Hence it suffices to encode in $\cE(\cK)$, the set $\cE\setminus\cK$.
At first we present a encoding scheme which encodes set $\cE_{(j,[x,y])}\setminus \cK_{(j,[x,y])}$ in prefix-free binary string $\cE_{(j,[x,y])}(\cK_{(j,[x,y])})$ for some good block $(j,[x,y])$, where $\cE_{(j,[x,y])}$ is the non-empty intervals in good block $(j,[x,y])$ and $\cK_{(j,[x,y])}\triangleq\cK\cap\cE_{(j,[x,y])}$.
Then we show that we can efficiently encode $\cE\setminus\cK$ block by block.

\subsection{A encoding scheme works within good block}
	\subsubsection{Encode $\cE_{(j,[x,y])}$ given $\cK_{(j,[x,y])},Q_{\pub}$}
	Let $K_{ne}\triangleq |\cE_{(j,[x,y])}|,K_{un}\triangleq |\cE_{(j,[x,y])}\setminus\cK_{(j,[x,y])}|$.
	Let $I_1,I_2,\ldots,I_{K_{ne}}\in\cE_{(j,[x,y])}$ be all the elements in the increasing order.
	Let $I_{i_1}, I_{i_2},\ldots,I_{i_{K_{un}}}\in \cE_{(j,[x,y])}\setminus\cK_{(j,[x,y])}$ be all the elements to be encoded, where $i_1<i_2<\ldots<i_{K_{un}}$.
	We first write down $K_{ne}$, then for $a=1,\ldots,K_{un}$, we do the following:
	\begin{enumerate}
	    \item write down $i_a-i_{a-1}$ ($i_0$ is assumed to be $0$);
	    \item write down $I_{i_a}-I_{i_a-1}$.
	\end{enumerate}
	All integers are encoded using the folklore prefix-free encoding which takes $O(\log N)$ bits to encode a non-negative integer $N$.
	This completes $\cE_{(j,[x,y])}(\cK_{(j,[x,y])})$.

	\subsubsection{Decode $\cE_{(j,[x,y])}$ given $\cE_{(j,[x,y])}(\cK_{(j,[x,y])})$ and $\cK_{(j,[x,y])},Q_{\pub}$}
	 We read $K_{ne}$ (which, together with $|\cK_{(j,[x,y])}|,Q_{\pub}$, determines $K_{un}$), and for $a=1,\ldots,K_{un}$, do the following:
	\begin{enumerate}
		\item read the next integer and recover $i_a$;
		\item for $i=i_{a-1}+1,\ldots,i_a-1$, let $I_i$ be the next element in $\cE_{(j,[x,y])}$ ($i_0$ is assumed to be $0$);
		\item read the next integer and recover $I_{i_a}$.
	\end{enumerate}
	Finally, for $i=i_{K_{un}}+1,\ldots,K_{ne}$, let $I_i$ be the next element in $\cE_{(j,[x,y])}$.
	This recovers all $I_1,\ldots,I_{K_{ne}}$, hence, decodes $\cE_{(j,[x,y])}$.

	\subsubsection{The length of $\cE_{(j,[x,y])}(\cK_{(j,[x,y])})$}
	Next, we analyze the expected length of $\cE_{(j,[x,y])}(\cK_{(j,[x,y])})$.
	$K_{ne}$ takes $O(\log \log B)$ bits to encode.
	Then for $a=1,\ldots,K_{un}$, $(i_a-i_{a-1})$ takes $O(\log (i_a-i_{a-1}))$ bits to encode.
	Since all these integers sum up to (at most) $K_{ne}$, by concavity of $\log$, the total number of bits used to encode $\{i_a-i_{a-1}\}$ is at most 
	\[
		O(K_{un}\cdot \log\frac{K_{ne}}{K_{un}}).
	\]
	Then by \cref{fact: inequality}, %
	the expected encoding length of all $i_a-i_{a-1}$ is at most
	\begin{equation}\label{eqn_length_1}
        O\left(\mathbb{E}[|\cE_{(j,[x,y])}\setminus\cK_{(j,[x,y])}|]\log\frac{\mathbb{E}[|\cE_{(j,[x,y])}|]}{\mathbb{E}[|\cE_{(j,[x,y])}\setminus\cK_{(j,[x,y])}|]}\right)
	\end{equation}

	Next, the value $I_{i_a}-I_{i_a-1}$ takes $O(\log (I_{i_a}-I_{i_a-1}))$ bits to encode.
	For all $a$ such that $I_{i_a}-I_{i_a-1}\le \left(\frac{\mathbb{E}[|\cE_{(j,[x,y])}|]}{\mathbb{E}[|\cE_{(j,[x,y])}\setminus\cK_{(j,[x,y])}|]}\right)^2$, their total encoding length is at most
	\[
		O\left(K_{un}\cdot \log\frac{\mathbb{E}[|\cE_{(j,[x,y])}|]}{\mathbb{E}[|\cE_{(j,[x,y])}\setminus\cK_{(j,[x,y])}|]}\right),
	\]
	and its expectation is at most
	\begin{equation}\label{eqn_length_2}
        O\left(\mathbb{E}[|\cE_{(j,[x,y])}\setminus\cK_{(j,[x,y])}|]\log\frac{\mathbb{E}[|\cE_{(j,[x,y])}|]}{\mathbb{E}[|\cE_{(j,[x,y])}\setminus\cK_{(j,[x,y])}|]}\right)
	\end{equation}

\begin{lemma}[{\cite[Lemma 17]{liu2020lower}}]\label{lem_large_gap}
	In a good block, for any $t\ge 1$, the expected number of non-empty interval pairs that have between $t-1$ and $2t$ empty intervals and no non-empty interval in between is at most $O\left(\sqrt{(\log^4B)/t}+1\right)$.
\end{lemma}
	For all $a$ such that $I_{i_a}-I_{i_a-1}> \left(\frac{\mathbb{E}[|\cE_{(j,[x,y])}|]}{\mathbb{E}[|\cE_{(j,[x,y])}\setminus\cK_{(j,[x,y])}|]}\right)^2$, by \cref{lem_large_gap}, the summation of their expected encoding lengths is at most
	\begin{align*}
		&\ \sum_{t=2^b\cdot\left(\frac{\mathbb{E}[|\cE_{(j,[x,y])}|]}{\mathbb{E}[|\cE_{(j,[x,y])}\setminus\cK_{(j,[x,y])}|]}\right)^2:b\geq 0, t\le \log^4B} O\left(\left(\sqrt{(\log^4B)/t}+1\right)\log t\right)\nonumber\\
		\le& O\left((\log^2B)\mathbb{E}[|\cE_{(j,[x,y])}\setminus\cK_{(j,[x,y])}|]/\mathbb{E}[|\cE_{(j,[x,y])}|]\cdot\log \left(\frac{\mathbb{E}[|\cE_{(j,[x,y])}|]}{\mathbb{E}[|\cE_{(j,[x,y])}\setminus\cK_{(j,[x,y])}|]}\right)+\log^2\log B\right).
	\end{align*}
    Since $\mathbb{E}[|\cE_{(j,[x,y])}|]=\Omega(\log^2B)$ by \cref{lem_entropy_lb}, it is at most
    \begin{align}
        O\left(\mathbb{E}[|\cE_{(j,[x,y])}\setminus\cK_{(j,[x,y])}|]\cdot\log \left(\frac{\mathbb{E}[|\cE_{(j,[x,y])}|]}{\mathbb{E}[|\cE_{(j,[x,y])}\setminus\cK_{(j,[x,y])}|]}\right)+\log^2\log B\right).\label{eqn_length_3}
    \end{align}

	Finally, summing up \eqref{eqn_length_1}, \eqref{eqn_length_2} and \eqref{eqn_length_3}, the expected length of $\cE_{(j,[x,y])}(\cK_{(j,[x,y])})$ is at most
	\[
        O\left(\mathbb{E}[|\cE_{(j,[x,y])}\setminus\cK_{(j,[x,y])}|]\cdot\log \left(\frac{\mathbb{E}[|\cE_{(j,[x,y])}|]}{\mathbb{E}[|\cE_{(j,[x,y])}\setminus\cK_{(j,[x,y])}|]}\right)+\log^2\log B\right).
	\]

	\subsection{Encoding $\cE\setminus\cK$}
	To encode $\cE$ given $\cK$, we just enumerate the good blocks in lexicographical order and write down the $\cE_{(j,[x,y])}(\cK_{(j,[x,y])})$ one by one.
	Let $\cG$ denote the set of good blocks.
	We calculate the expected cost to complete the proof:
	\begin{align*}
		\mathbb{E}\left[\sum_{(j,[x,y])\in\cG}\left(\mathbb{E}[|\cE_{(j,[x,y])}\setminus\cK_{(j,[x,y])}|]\cdot\log \left(\frac{\mathbb{E}[|\cE_{(j,[x,y])}|]}{\mathbb{E}[|\cE_{(j,[x,y])}\setminus\cK_{(j,[x,y])}|]}\right)+\log^2\log B\right)\right].
	\end{align*}
	By applying the law of total expectation, we can restrict the distribution to the event that $\cG\ne\emptyset$.
	We let $(j,[x,y])\sim\cG$ denote we sample $(j,[x,y])$ from $\cG$ uniformly at random.
	\begin{align*}
		&\mathbb{E}\left[|\cG|\cdot\left(\mathbb{E}_{(j,[x,y])\sim\cG}\left[\mathbb{E}[|\cE_{(j,[x,y])}\setminus\cK_{(j,[x,y])}|]\cdot\log \left(\frac{\mathbb{E}[|\cE_{(j,[x,y])}|]}{\mathbb{E}[|\cE_{(j,[x,y])}\setminus\cK_{(j,[x,y])}|]}\right)\right]+\log^2\log B\right)\right]
		\intertext{Observe that $\mathbb{E}_{(j,[x,y])\sim\cG}\left[\mathbb{E}[|\cE_{(j,[x,y])}\setminus\cK_{(j,[x,y])}|]\right]=\mathbb{E}[|\cE\setminus\cK|]/|\cG|$ and $\mathbb{E}_{(j,[x,y])\sim\cG}\left[\mathbb{E}[|\cE_{(j,[x,y])}|]\right]=\mathbb{E}[|\cE|]/|\cG|$. By \cref{fact: inequality},}
		\le&\mathbb{E}[|\cE\setminus\cK|]\log(\mathbb{E}[|\cE|]/\mathbb{E}[|\cE\setminus\cK|])+\mathbb{E}[|\cG|\cdot\log^2\log B].
	\end{align*}
	The lemma then follows from the fact that $|\cG|\le p$.

\ifx\mainfile\undefined
\bibliography{refs}
\bibliographystyle{alpha}
\end{document}
\fi
